# Supplementary material for: CBCT-to-CT synthesis with a single neural network for head-and-neck, lung and breast cancer adaptive radiotherapy
Source: arXiv:1912.11136 source file (2019-12-23)
Supplement: Supplementary file 1 [file SuppMat.pdf]

# Supplementary Material

"CBCT-to-CT synthesis with a single deep learning network for head-and-neck, lung and breast cancer adaptive radiotherapy"


**Abstract**

This file contains the supplementary material reporting: a collection of patient demographics 1, and an overview of additional metric for the image comparison 2.


## 1. Patient demographic

Sex, age, tumour type, tumour stage, dose prescription in terms of total dose, fractionation scheme, linac on which the CBCT have been acquired and day between CBCT and CT were reported for all the patients in the training, validation and test set for head-and-neck (Tab. 1), breast (Tab. 2) and lung (Tab. 3). For the patients in the training set, the CBCT have been the closest to CT or rCT. For the patients in the test set, the RT plan was briefly described in terms of angle of the beam and the arc of irradiation for intensity-modulated radiotherapy (IMRT) and volumetric modulated arc therapy (VMAT), respectively. Also, the volumetric percentage difference of the body between rCT ($\Delta V_{\text{rCT}}$) and sCT ($\Delta V_{\text{sCT}}$) to CT in $\text{Mask}_{\text{FOV}}$ was reported.

Table 1: Overview of the patients demographic for the **head-and-neck** cancer patients split in training, validation and test set.

| Set | Pt no. | Sex | Age [y] | Tumour | Stage [TNM] | Prescription | Frac no. | Dose per frac. [Gy] | Plan* | Linac | CBCT-to-(r)CT [d] | rCT-to-CT [d] | $\Delta V_{rCT}$ [%] | $\Delta V_{sCT}$ [%] |
|---|---|---|---|---|---|---|---|---|---|---|---|---|---|---|
| Training | H1 | M | 60.4 | Oropharynx R | T3N2b | 70Gy SIB | 35 | 2.0 | | U09 | 3 | | | |
| | H2 | M | 67.3 | Larynx glottid | cT1aN0 | 60Gy | 25 | 2.4 | | U11 | 1 | | | |
| | H3 | M | 48.1 | Tongue R | pT4aN2b | 66Gy SIB | 33 | 2.0 | | U14 | 3 | | | |
| | H4 | M | 68.6 | Larynx | pT4cN0 | 66Gy SIB | 33 | 2.0 | | U14 | 32[a] | | | |
| | H5 | M | 62.7 | Nasopharynx | cTxN2cMx | 70Gy SIB | 35 | 2.0 | | U14 | 0 | | | |
| | H6 | M | 58.6 | Nasopharynx | T1N2 | 70Gy SIB | 35 | 2.0 | | U11 | 4 | | | |
| | H7 | M | 71.6 | Oropharynx | T2N3 | 70Gy | 35 | 2.0 | | U14 | 1 | | | |
| | H8 | M | 54.5 | Oropharynx | T4aN2cM0 | 46Gy, boost 70Gy | 23 | 2.0 | | U14 | 2 | | | |
| | H9 | M | 53.6 | Tonsil | T2N2aM0 | 70Gy SIB | 35 | 2.0 | | U11 | 0 | | | |
| | H10 | M | 69.7 | Parotis L (meths SCC) | T4NxM1 | 66Gy adjuv | 33 | 2.0 | | U14 | 4 | | | |
| | H11 | M | 49.0 | Oropharynx R | cT1cN2acM0 | 70Gy SIB | 35 | 2.0 | | U09 | 3 | | | |
| | H12 | M | 66.8 | Oropharynx (tonsil) | cT2N2b | 70Gy SIB | 35 | 2.0 | | U11 | 2 | | | |
| | H13 | F | 70.5 | Parotis L | T1aN0 | 50Gy | 25 | 2.0 | | U14 | 4 | | | |
| | H14 | F | 61.3 | Hypopharynx R | T2N1M0 | 46Gy SIB | 23 | 2.0 | | U14 | 5 | | | |
| | H15 | F | 52.3 | Nasopharynx | cT3N2bM0 | 46Gy SIB | 23 | 2.0 | | U14 | 2 | | | |
| Validation | H16 | M | 74.6 | Tonguebasis | T4N2c | 70Gy SIB | 35 | 2.0 | | U14 | 0 | 261 | | |
| | H17 | M | 67.3 | SupraClav R | cT4N3M1 | 16Gy reirr | 2 | 8.0 | | U05 | 0 | | | |
| | H18 | F | 54.3 | Hypopharynx axilla R | cT1N3M1 | 70Gy | 35 | 2.0 | | U14 | 10 | 34 | | |
| | H19 | M | 85.6 | Tonsil epiglottis | T2N1 | 69Gy | 30 | 2.3 | | U11 | 12 | 121 | | |
| | H20 | M | 74.5 | Non-Hodgkin Lymph SupraClav L | Deauville V | 30Gy pall | 10 | 3.0 | | U12 | 3 | | | |
| | H21 | M | 67.3 | Tongue R | cT1N2bM1 | 48Gy prim + lymph | 16 | 3.0 | | U12 | 16 | | | |
| | H22 | F | 53.5 | Hypopharynx SIB | T4a | 70Gy SIB | 35 | 2.0 | | U12 | -6 | 32 | | |
| | h23 | F | 71.4 | Head L | cT3N2M1b | 20Gy pall reirr | 5 | 4.0 | | U05 | 4 | | | |
| Test | H24 | M | 71.4 | Hypopharynx L | T4aN2b | 70Gy SIB | 35 | 2.0 | 360° | U09 | 55 | 56 | -7.8 | -8.0 |
| | H25 | M | 64.0 | Head R | T3N1 | 46Gy | 23 | 2.0 | 360° | U11 | 47 | 47 | -9.7 | -9.6 |
| | H26 | M | 67.3 | Supraglottis | T2N0M0 | 70Gy SIB | 35 | 2.0 | 360° | U14 | 63 | 64 | -6.6 | 6.1 |
| | H27 | F | 74.7 | Parotis L | pT3N2b | 47Gy SIB | 15 | 1.8 | 360° | U14 | 16 | 20 | -3.1 | -3.0 |
| | H28 | M | 55.3 | Oropharynx | T2N0M0 | 70Gy SIB | 12/35 | 2.0 | 180° | U15 | 53 | 49 | -2.7 | -3.3 |
| | H20 | M | 62.0 | Oropharynx | cT4aN2c | 47Gy SIB | 15 | 1.8 | 180° | U12 | 44 | 44 | -4.0 | -4.6 |
| | H30 | M | 61.2 | Parotis R | cT0N2aM0 | 69Gy | 3/33 | 2.3 | 170° | U11 | 43 | 35 | -1.8 | -2.3 |
| | H31 | M | 52.0 | Oropharynx L tongue L | cT4N3bM0 | 70Gy SIB | 35 | 2.0 | 360° | U10 | 39 | 34 | -0.3 | -1.1 |
| | H32 | F | 53.7 | Mouth bed SIB | pT4acN0M0 | 70Gy adjuv | 12/35 | 2.0 | 170° | U14 | 67 | 62 | 1.6 | 1.5 |
| | H33 | M | 75.5 | Glottis Larynx R | cT2N0M0 | 70Gy | 35 | 2.0 | 360° | U10 | 34 | 34 | -8.0 | -8.3 |

*VMAT plans with 6 MV energy were generally delivered plans indicates the degree of the arc. [a] In this case the days can between CBCT and CT. Abbreviations: R = right; L = left; SIB = simultaneous integrated boost; reirr = reirradiation; pall = palliation; adjuv = adjuvant therapy; SupraClav = supra clavicular; SCC = squamous cell carcinoma; lymph = lymphonode irradiation; $\Delta V_{rCT}$ = percentage difference of the volume in $Mask_{CBCT}$ of the body calculated in rCT respect to CT; $\Delta V_{rCT}$ = percentage difference of the volume in $Mask_{CBCT}$ of the body calculated in sCT respect to CT.

Table 2: Overview of the patients demographic for **breast** cancer patients split in training, validation and test set.

| Set | Pt no. | Sex | Age [y] | Tumour | Stage [TNM] | Prescription | Frac no. | Dose per frac. [Gy] | Plan* | Linac | CBCT-to-(r)CT [d] | rCT-to-CT [d] | $\Delta V_{rCT}$ [%] | $\Delta V_{sCT}$ [%] |
|---|---|---|---|---|---|---|---|---|---|---|---|---|---|---|
| Training | B1 | F | 57.6 | R | cT2-3N2M0 | 42.56Gy | 16 | 2.66 | | U10 | 0 | | | |
| | B2 | F | 33.3 | L locoreg | cT3N1M0 | 61.2Gy SIB + lymph | 23 | 2.66 | | U12 | 1 | | | |
| | B3 | F | 46.6 | R local | pT1cN1 | 46Gy SIB | 21 | 2.66 | | U12 | 5 | | | |
| | B4 | F | 52.2 | R local | cT2N0M0 | 46Gy SIB | 21 | 2.66 | | U11 | 2 | | | |
| | B5 | F | 45.8 | R | cT2N0M0 | 46Gy SIB | 21 | 2.66 | | U05 | 5 | | | |
| | B6 | F | 63.3 | R locoreg | cT2N1M0 | 46Gy | 21 | 2.66 | | U14 | 4 | | | |
| | B7 | F | 59.5 | R | pT2N0 | 42.56Gy reirr | 16 | 2.66 | | U04 | 5 | | | |
| | B8 | F | 84.9 | R | pT2N3M0 | 61.2Gy SIB | 23 | 2.66 | | U11 | 2 | | | |
| | B9 | F | 60.0 | R | cT2N2M0 | 46Gy SIB | 21 | 2.66 | | U04 | 4 | | | |
| | B10 | F | 66.7 | L locoreg | cT2N2M0 | 42.56Gy | 16 | 2.66 | | U11 | 5 | | | |
| | B11 | F | 67.1 | R | pT1G2N0 | 42.56Gy | 16 | 2.66 | | U04 | 1 | | | |
| | B12 | F | 69.4 | L local | cT2N0Mx | 46Gy SIB + 21x0.5 seq | 21 | 2.66 | | U11 | 4 | | | |
| | B13 | F | 93.7 | R | pT1N1 | 24Gy pall | 3 | 8.00 | | U04,U10 | 2 | | | |
| | B14 | F | 67.7 | R | cT2-3N2M0 | 42.56Gy | 16 | 2.66 | | U04,U07 | 4 | | | |
| | B15 | F | 37.1 | R | cT1N0 | 46Gy SIB | 21 | 2.66 | | U04 | 4 | | | |
| Validation | B16 | F | 56.5 | R postop | pT1N0 | 55.86Gy SIB | 21 | 2.17 | | U10 | 14 | / | | |
| | B17 | F | 57.2 | Thorax | T23 | 45.57 local | 21 | 2.17 | | U12 | -7 | 54 | | |
| | B18 | F | 63.5 | R | cT2pN1M0 | 46Gy SIB neo-adjuv chemo | 23 | 2.66 | | U04 | 7 | 49 | | |
| | B19 | F | 69.5 | R preop | pT1aN0 | 42.56Gy | 16 | 2.66 | | U04 | 38 | 27 | | |
| | B20 | F | 70.0 | L | pT4N0 | 60Gy SBRT | 5 | 12.00 | | U09 | 47 | 187 | | |
| | B21 | F | 67.7 | R postop | cT2-3N2M0 | 42.56Gy adj | 16 | 2.66 | | U04,U07 | 1 | 44 | | |
| | B22 | F | 52.4 | R | pT1cG2N1 | 42.56Gy | 16 | 2.66 | | U05 | 7 | 9-25 | | |
| | B23 | F | 67.6 | L | cT1cN0 | 15/20Gy SIB | 1 | 20.00 | | U10 | 8 | | | |
| Test | B24 | F | 76.8 | R postop | pT1cN0 | 61.2Gy SIB | 23 | 2.66 | 6MV 8f* | U04 | 14 | 14 | 3.6 | 6.8 |
| | B25 | F | 50.3 | L postop | pT1N0 | 61.2Gy SIB | 23 | 2.66 | 10MV 7f* | U14 | 26 | 26 | 5.4 | 5.5 |
| | B26 | F | 72.2 | L postop | pT1cG2N1 | 42.56Gy lymph | 16 | 2.66 | 10MV 4f* | U08 | 16 | 14 | 3.5 | 3.6 |
| | B27 | F | 77.3 | L local | pT3N1 | 61.2Gy SIB | 23 | 2.66 | 6/10MV 4/8f* | U14 | 23 | 22 | -3.5 | 2.7 |
| | B28 | F | 43.8 | R Thoraxwand locoreg | cT2mN3bM0 | 42.56Gy | 16 | 2.66 | 10MV 270° | U14 | 8 | 11 | -1.0 | -0.4 |
| | B29 | F | 74.1 | R locoreg | pT1cpN2 | 42.56Gy lymph | 16 | 2.66 | 6/10MV 2/9f* | U04 | 21 | 21 | -1.6 | -1.7 |
| | B30 | F | 57.8 | L local | cT2N1M0 | 42.56Gy | 16 | 2.66 | 10MV 10f* | U11 | 17 | 17 | 8.3 | 9.3 |
| | B31 | F | 72.2 | L postop | pT1cG2N1 | 42.56Gy lymph | 16 | 2.66 | 6MV 220° | U11 | 14 | 12 | -2.8 | -2.7 |
| | B32 | F | 39.2 | L boost | pT1cN0M0 | 40.05Gy | 15 | 2.67 | 6MV 240° | U12 | 20 | 20 | -8.2 | -13.9 |
| | B33 | F | 42.3 | L postop | cT1bN0/1 | 40.05Gy | 15 | 2.67 | 6/10MV 4/5f* | U12 | 31 | 28 | 0.9 | -0.4 |

* f = fields/beams of IMRT; if f is not indicated, a VMAT plan was delivered and the arc range is expressed in degree. Abbreviations: R = right; L = left; SIB = simultaneous integrated boost; reirr = reirradiation; pall = palliation; (neo) adjuv = (neo)adjuvant therapy; chemo = chemotherapy; seq = sequential; local = local treatment; locoreg = locoregional treatment; postop = postoperative irradiation; lymph = lymphonode irradiation; $\Delta V_{rCT}$ = percentage difference of the volume in $Mask_{CBCT}$ of the body calculated in rCT respect to CT; $\Delta V_{rCT}$ = percentage difference of the volume in $Mask_{CBCT}$ of the body calculated in sCT respect to CT.

Table 3: Overview of the patients demopgraphic for the **lung** cancer patients split in training, validation and test set.

| Set | Pt no. | Sex | Age [y] | Tumour | Stage [TNM] | Prescription | Frac no. | Dose per frac. [Gy] | Plan* | Linac | CBCT-to-(r)CT [d] | rCT-to-CT [d] | $\Delta V_{\mathrm{rCT}}$ [%] | $\Delta V_{\mathrm{sCT}}$ [%] |
|---|---|---|---|---|---|---|---|---|---|---|---|---|---|---|
| Training | L1 | F | 55.2 | R NSCLC R | cT4N2M1a | 16Gy pall | 2 | 8.00 | | U05 | 0 | | | |
| | L2 | F | 77.8 | NSCLC R | pT2bN3M1a-b | 8Gy pall | 1 | 8.00 | | U05 | 0 | | | |
| | L3 | M | 80.5 | R | T4 | 8Gy pall | 1 | 8.00 | | U04 | 0 | | | |
| | L4 | F | 52.7 | R NSCLC recidive | T4 | 8Gy pall | 1 | 8.00 | | U05,U03 | 0 | | | |
| | L5 | F | 59.5 | Adenocarc postop | T4N1M1 | 30Gy | 10 | 3.00 | | U04,U05 | 18 | | | |
| | L6 | F | 59.9 | Meths | T2-3 | 30Gy | 10 | 3.00 | | U09,U05 | 4 | | | |
| | L7 | F | 60.3 | Adenocarc R | pT1N0Mo | 60Gy SBRT | 5 | 12.00 | | U09 | 2 | | | |
| | L8 | F | 61.2 | R + meths | T2-3 | 30Gy | 10 | 3.00 | | U09 | 4 | | | |
| | L9 | M | 69.8 | R Thoraxwand | T4N2M1c | 8Gy | 1 | 8.00 | | U04 | 0 | | | |
| | L10 | M | 65.1 | L | pT4aN0M0 | 8Gy reirr | 1 | 8.00 | | U05 | 1 | | | |
| | L11 | M | 55.7 | L NSCLC | T4 | 20Gy | 5 | 4.00 | | U11 | 1 | | | |
| | L12 | M | 83.9 | L NSCLC | cT4N0Mo | 39Gy | 13 | 3.00 | | U09,U14 | 1 | | | |
| | L13 | M | 60.6 | L NSCLC | cT4N1M1c | 8Gy pall | 1 | 8.00 | | U05 | 0 | | | |
| | L14 | M | 63.3 | SCLC | cT2N2M0 | 39Gy | 13 | 3.00 | | U09 | 3 | | | |
| | L15 | M | 59.7 | R NSCLC | cT4N4M1a | 8Gy pall | 1 | 8.00 | | U05 | 0 | | | |
| Validation | L16 | M | 70.6 | Mediastinum | pT4N2M0 | 65Gy | 25 | 3.00 | | U12 | -25 | 36 | | |
| | L17 | M | 59.4 | R NSCLC | cT4N3M1 | 48Gy | 16 | 3.00 | | U9 | -9 | 13 | | |
| | L18 | M | 62.5 | L SCLC | cT3N3M0 | 45 Gy SIB | 15 | 5.00 | | U12 | 0 | 78 | | |
| | L19 | M | 59.8 | L NSCLC | T4 | 16Gy pall | 2 | 8.00 | | U09 | 5 | / | | |
| | L20 | M | 74.4 | L SCLC | T4 | 8Gy | 1 | 8.00 | | U04 | 0 | 159 | | |
| | L21 | M | 56.5 | R NSCLC local | pT3N1M0 | 54 Gy pall | 3 | 18.00 | | U12 | 11 | / | | |
| | L22 | F | 8.9 | Wilms, both | T1 | 12Gy+22Gy SIB | 8 | 1.5+2.75 | | U15 | 14 | / | | |
| | L23 | M | 63.2 | L | cT2N2M0 | 60Gy SBRT | 8 | 7.50 | | U15 | 24 | 25 | | |
| Test | L24 | M | 64.0 | Adenocarc | cT1cN2M0 | 65Gy | 25 | 2.60 | 10MV 195° | U11 | 27 | 28 | 2.5 | -1.8 |
| | L25 | F | 60.9 | NSCLC | cT2N3M0 | 65 Gy | 25 | 2.60 | 10MV 195° | U10 | 21 | 21 | -4.2 | -2.3 |
| | L26 | F | 67.0 | L SCLC | cT4N3M1c | 30Gy SABRT | 10 | 3.00 | 10MV 195° | U14 | 11 | 11 | 5.3 | -0.3 |
| | L27 | M | 81.7 | L locoreg | T4N2M0 | 36Gy SABRT | 12 | 3.00 | 10MV 195° | U12 | 12 | 14 | -2.6 | -5.8 |
| | L28 | M | 82.3 | R | cT1aN0M0 | 65Gy | 25 | 2.60 | 10MV 195° | U14 | 23 | 23 | -1.4 | 0.0 |
| | L29 | F | 57.5 | Adenocarc R | T2N4 | 60Gy SABRT | 5 | 12.00 | 6MV 360° | U04 | 27 | 27 | 1.3 | 2.8 |
| | L30 | M | 63.3 | SCLC | cT2N2M0 | 66Gy | 33 | 2.00 | 10MV 195° | U09 | 8 | 12 | 2.9 | 3.4 |
| | L31 | M | 81.8 | Adenocarc R | c3T3N3M0 | 3Gy pall | 10 | 3.0 | 10MV 2f* | U14 | -47 | -49 | 0.4 | 1.1 |
| | L32 | F | 73.1 | R NSCLC | T3N2M0 | 65Gy | 25 | 2.60 | 10MV 195° | U15 | 14 | 16 | -1.1 | -1.4 |
| | L33 | F | 60.8 | L NSCLC | T4N1M0 | 65Gy | 25 | 2.60 | 10MV 195° | U08 | 22 | 24 | 0.4 | 0.5 |

* f = fields/beams of IMRT; if f is not indicated, a VMAT plan was delivered and the arc range is expressed in degree. Abbreviations: R = right; L = left; both = both lungs were irradaited; SIB = simultaneous integrated boost; NSCLC = Non-small-cell lung carcinoma; SCLC = Small-cell lung carcinoma; reirr = reirradiation; pall = palliation; SABRT = stereotactic ablative radiotherapy; SBRT = stereotactic body radiation therapy ; postop = postoperative irradiation; adenocarc = adenocarcinoma; $\Delta V_{\mathrm{rCT}}$ = percentage difference of the volume in $\mathrm{Mask}_{\mathrm{CBCT}}$ of the body calculated in rCT respect to CT; $\Delta V_{\mathrm{rCT}}$ = percentage difference of the volume in $\mathrm{Mask}_{\mathrm{CBCT}}$ of the body calculated in sCT respect to CT.

## 2. Image Comparison

Table 4 reports the similarity between the intensity of sCT, CBCT, CT and rCT calculated within $\text{Mask}_{\text{CBCT}}$ in terms of peak signal-to-noise ratio (PSNR) and structural similarity index metric (SSIM) as proposed by Liang et al. [1].

Table 4: Image comparison calculated as mean ($\pm 1\sigma$) and range ([min; max]) of the test dataset (30 patients) compared to the reference dataset in terms of peak signal-to-noise ratio (PSNR) and structural similarity index metric (SSIM) between the Test and the Ref images. Values are expressed in dB for the PSNR.

| Site | | Head-and-Neck | | Breast | | Lung | |
|---|---|---|---|---|---|---|---|
| **Test** | **Ref** | **PSRN** [dB] | **SSIM** | **PSNR** [dB] | **SSIM** | **PSNR** [dB] | **SSIM** |
| CBCT | rCT | 24.6±0.8 [23.1;26.1] | 0.46±0.05 [0.38;0.52] | 25.3±1.8 [22.2;28.1] | 0.71±0.04 [0.63;0.75] | 23.7±1.4 [22.2;26.7] | 0.69±0.04 [0.58;0.73] |
| sCT[1] | rCT | 30.5±2.2 [27.0;33.4] | 0.81±0.04 [0.75;0.88] | 29.0±2.1 [26.0;32.3] | 0.76±0.02 [0.72;0.79] | 28.5±1.6 [25.6;31.3] | 0.78±0.04 [0.72;0.88] |
| sCT* | rCT | 30.6±2.2 [27.1;33.7] | 0.80±0.04 [0.74;0.85] | 28.8±2.0 [25.7;31.8] | 0.80±0.04 [0.74;0.85] | 28.4±1.4 [26.1;31.1] | 0.78±0.05 [0.72;0.87] |
| CT | rCT | 27.9±1.9 [25.3;30.5] | 0.86±0.04 [0.80;0.92] | 28.2±2.3 [23.6;30.7] | 0.85±0.05 [0.74;0.90] | 27.0±1.9 [23.5;29.5] | 0.77±0.06 [0.63;0.83] |

[1] sCT obtained from a single network trained on all the anatomical sites.
* sCT obtained from three different networks trained on each anatomical site.

## 3. Single patient overview

In the following pages are shown CBCT, CT, rCT and sCT as well as the image differences to CT, dose, dose differences and DVH for the patients in the test set for whom analysis of DVH-points reported dose differences > 2% (B31, L25, L27). Multiple views (e.g. axial, sagittal or coronal) are presented according to which view was most representative to explain the differences reported.

In Figure 1 and 2, one can observe that anatomical differences due to residual set-up differences were present for B30 and B31, respectively. Specifically, for B30, a bolus was used, and it is evident the anatomical mismatch and difference in bolus position between rCT and sCT.

Figure 3 and Figure 4 report images and doses for lung cancer patiens L25 and L27, respectively. For both the patients, differnet respiratory phases can be notice. In addition, for L25, residual artefact characterised by inhomogeneous HUs seem to be present along the cranio-caudal direction in the lungs; it seems that for this case the CBCT artefacts were not fully recovered in the lungs. The image protocols were reconsidered for L25, and it was observed that this was the only patient acquired on the linac named "U10": no training data were present for lung patients from this linac. We hypothesise that data in the test may have been imbalanced compared to data in training set for what concern linacs.

For L27, one can observe that the CBCT was characterised by severe scatter artefacts probably because the patient was obese and the image protocol has not been optimised. In this case, bones on sCT were not entirely recovered, probably due to the low quality of CBCT.

## References

[1] X. Liang, L. Chen, D. Nguyen, Z. Zhou, X. Gu, M. Yang, J. Wang, S. Jiang, Generating synthesized computed tomography (CT) from cone-beam computed tomography (CBCT) using CycleGAN for adaptive radiation therapy, Phys. Med. Biol. 64 (12) (2019) 125002. doi:10.1088/1361-6560/ab22f9.

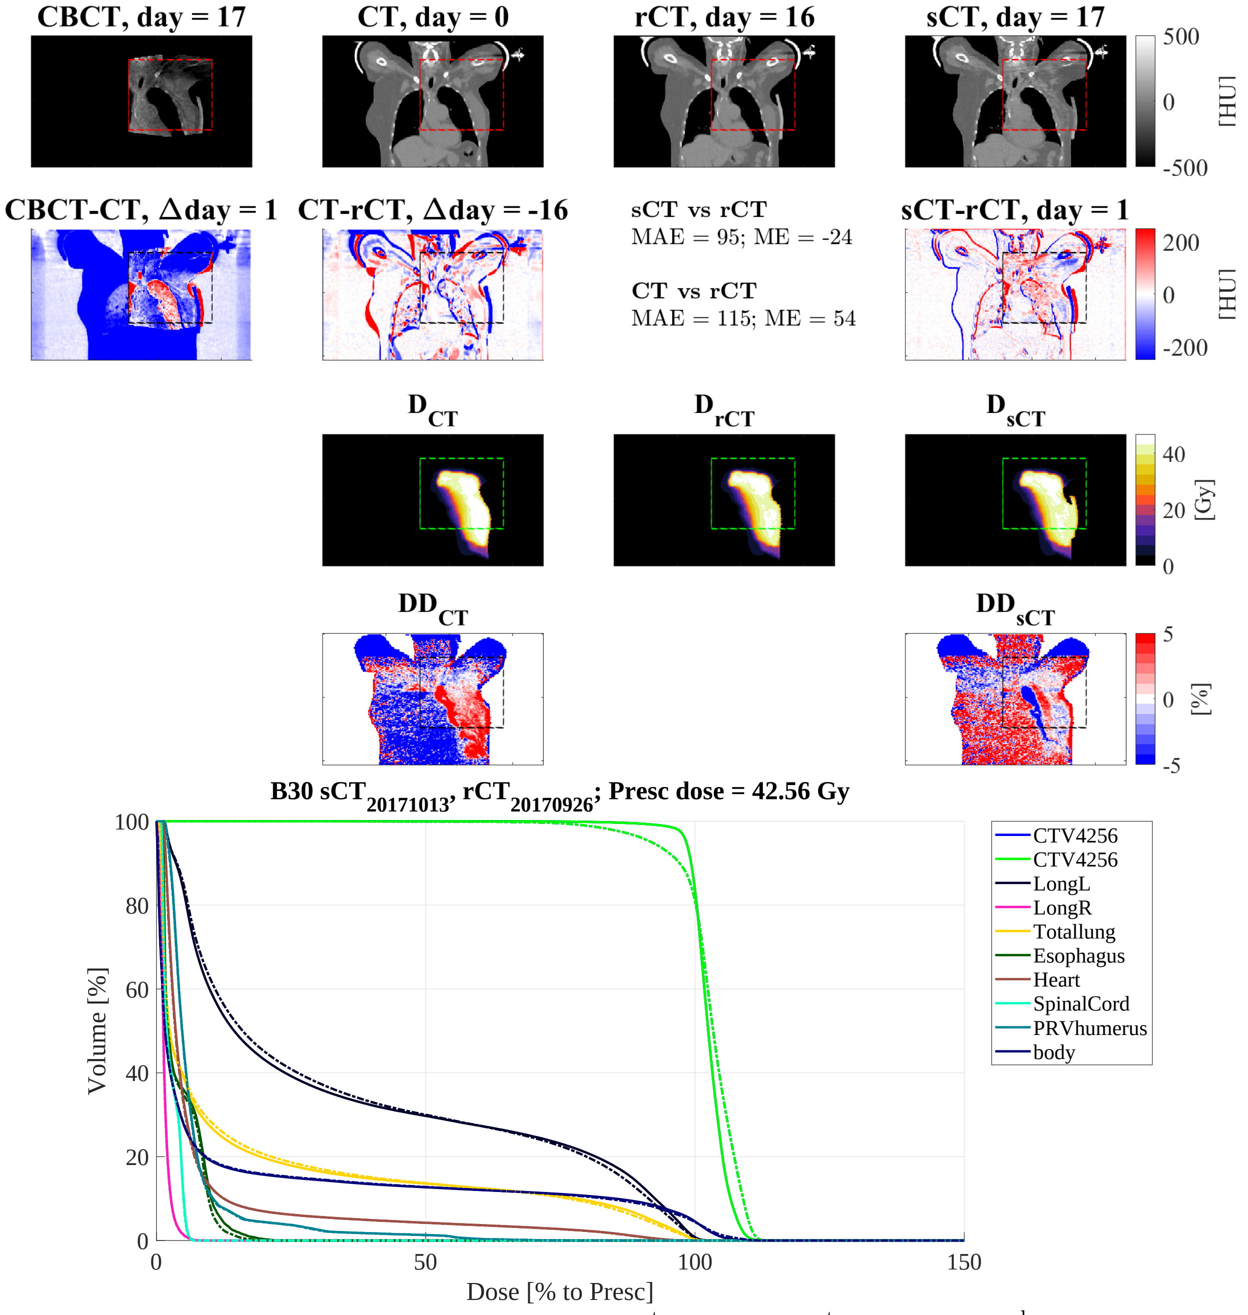


Figure 1: Coronal views for the breast cancer patient B30 of: (1st row) CBCT (1st column), CT (2nd column), rescan CT (rCT, 3rd column) and synthetic CT (sCT, 4th column), along with (2nd row) the respective difference to rCT, the doses (3rd row) and the relative dose differences (4th). The red, black, or green dotted rectangles indicate the position of $\mathrm{Mask}_{\mathrm{CBCT}}$. The days refer to the acquisition date of the rCT. In the 5th rows, the DVH is shown for target and OARs of sCT (continuous lines) and rCT (dashed lines).

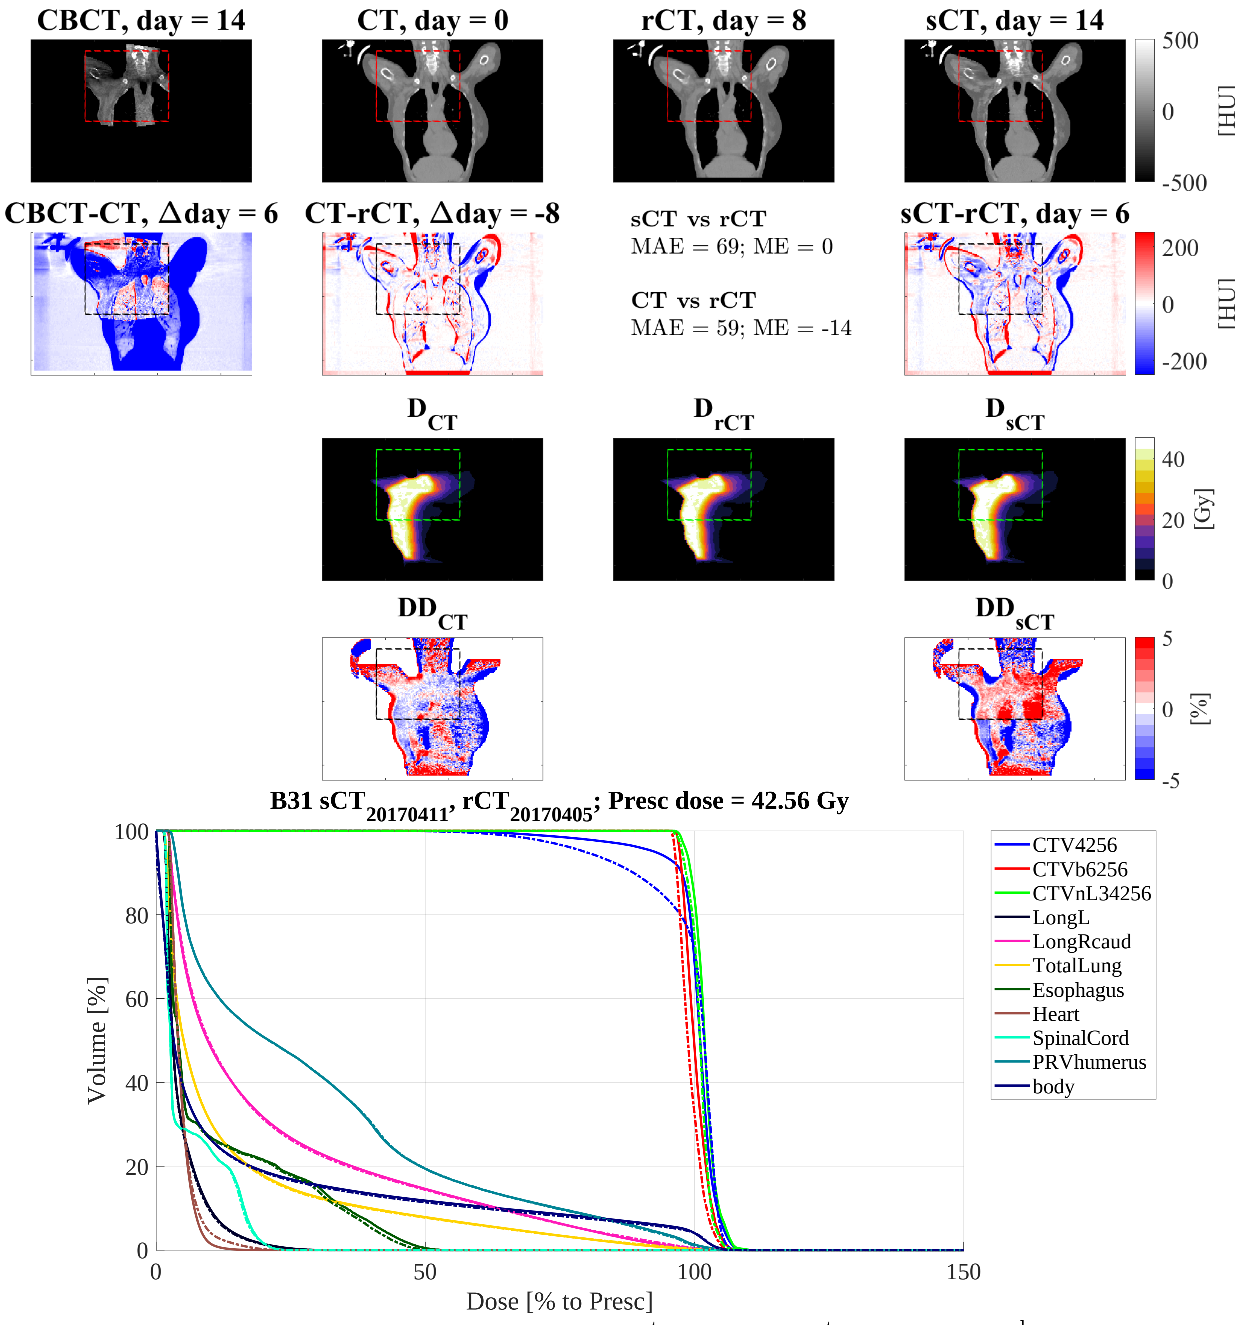


Figure 2: Coronal views for the breast cancer patient B31 of: ($1^{st}$ row) CBCT ($1^{st}$ column), CT ($2^{nd}$ column), rescan CT (rCT, $3^{rd}$ column) and synthetic CT (sCT, $4^{th}$ column), along with ($2^{nd}$ row) the respective difference to rCT, the doses ($3^{rd}$ row) and the relative dose differences ($4^{th}$). The red, black, or green dotted rectangles indicate the position of $\text{Mask}_{\text{CBCT}}$. The days refer to the acquisition date of the rCT. In the $5^{th}$ rows, the DVH is shown for target and OARs of sCT (continuous lines) and rCT (dashed lines).

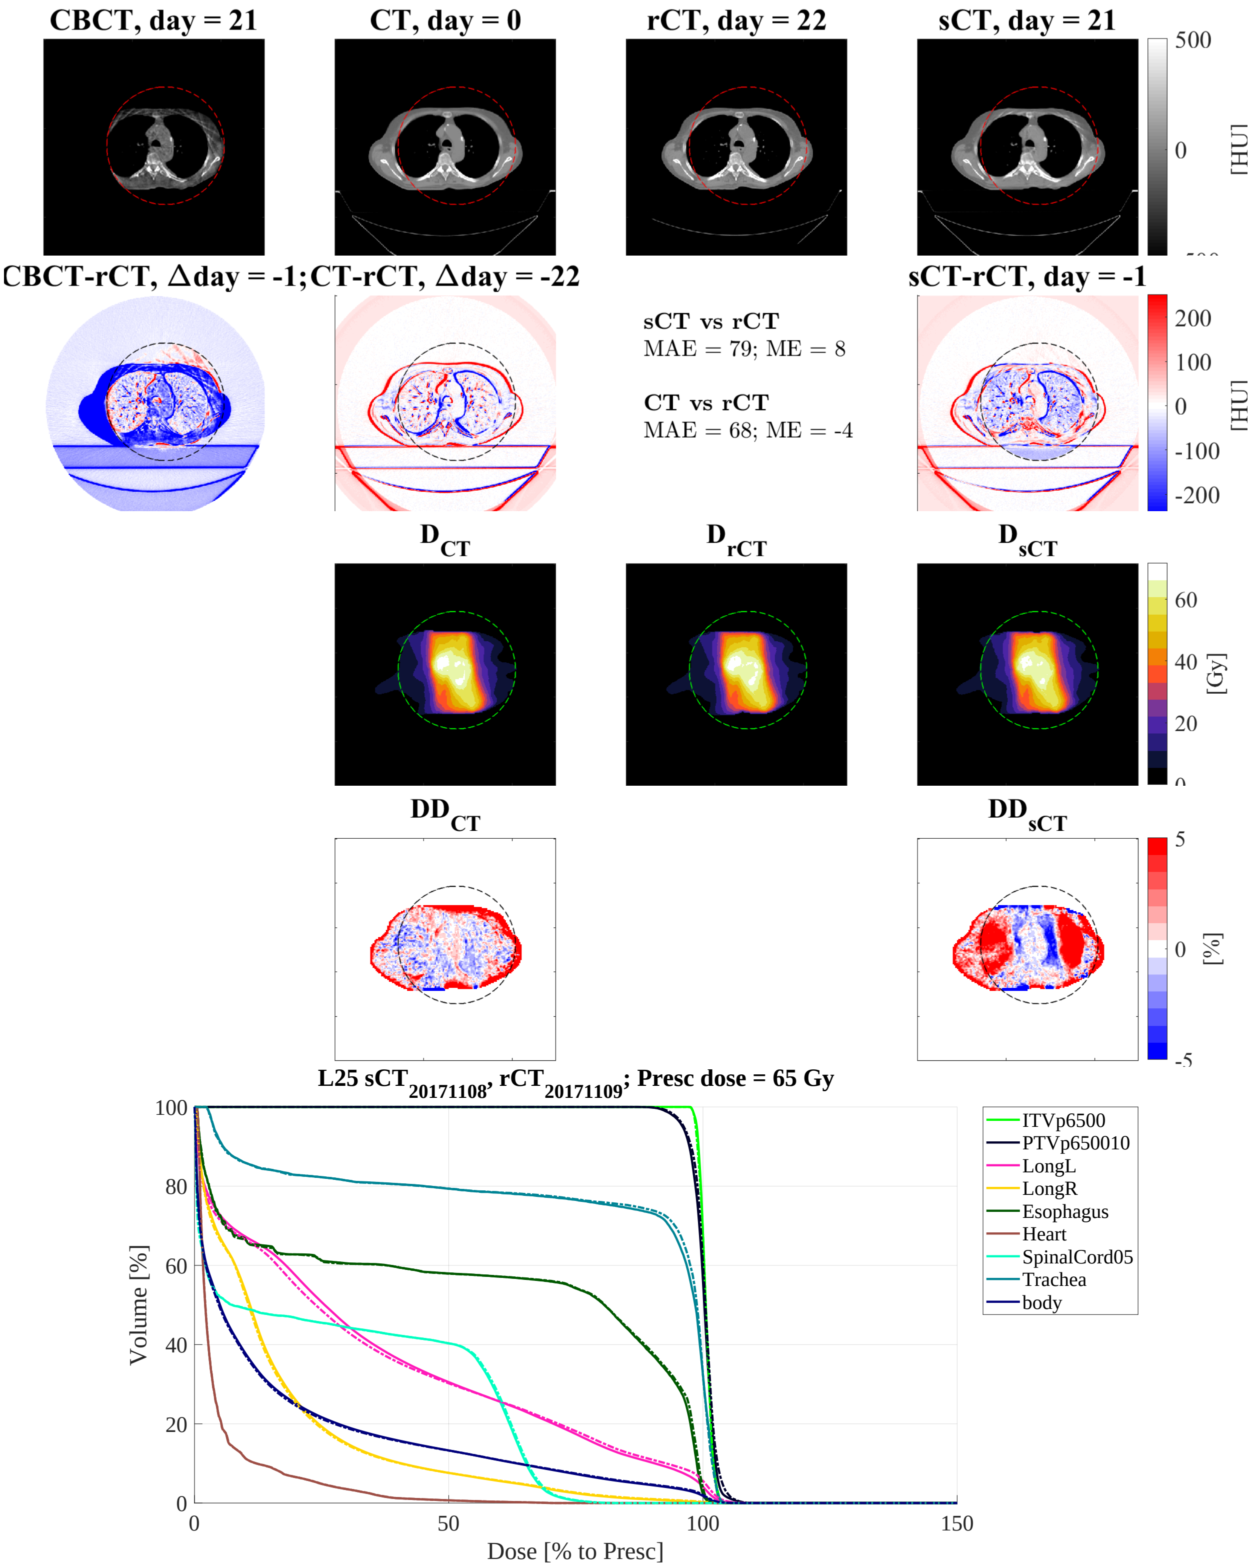


Figure 3: Axial views for the lung cancer patient L25 of: (1st row) CBCT (1st column), CT (2nd column), rescan CT (rCT, 3rd column) and synthetic CT (sCT, 4th column), along with (2nd row) the respective difference to rCT, the doses (3rd row) and the relative dose differences (4th). The red, black, or green dotted rectangles indicate the position of $\text{Mask}_{\text{CBCT}}$. The days refer to the acquisition date of the rCT. In the 5th row, the DVH is shown for target and OARs of sCT (continuous lines) and rCT (dashed lines).

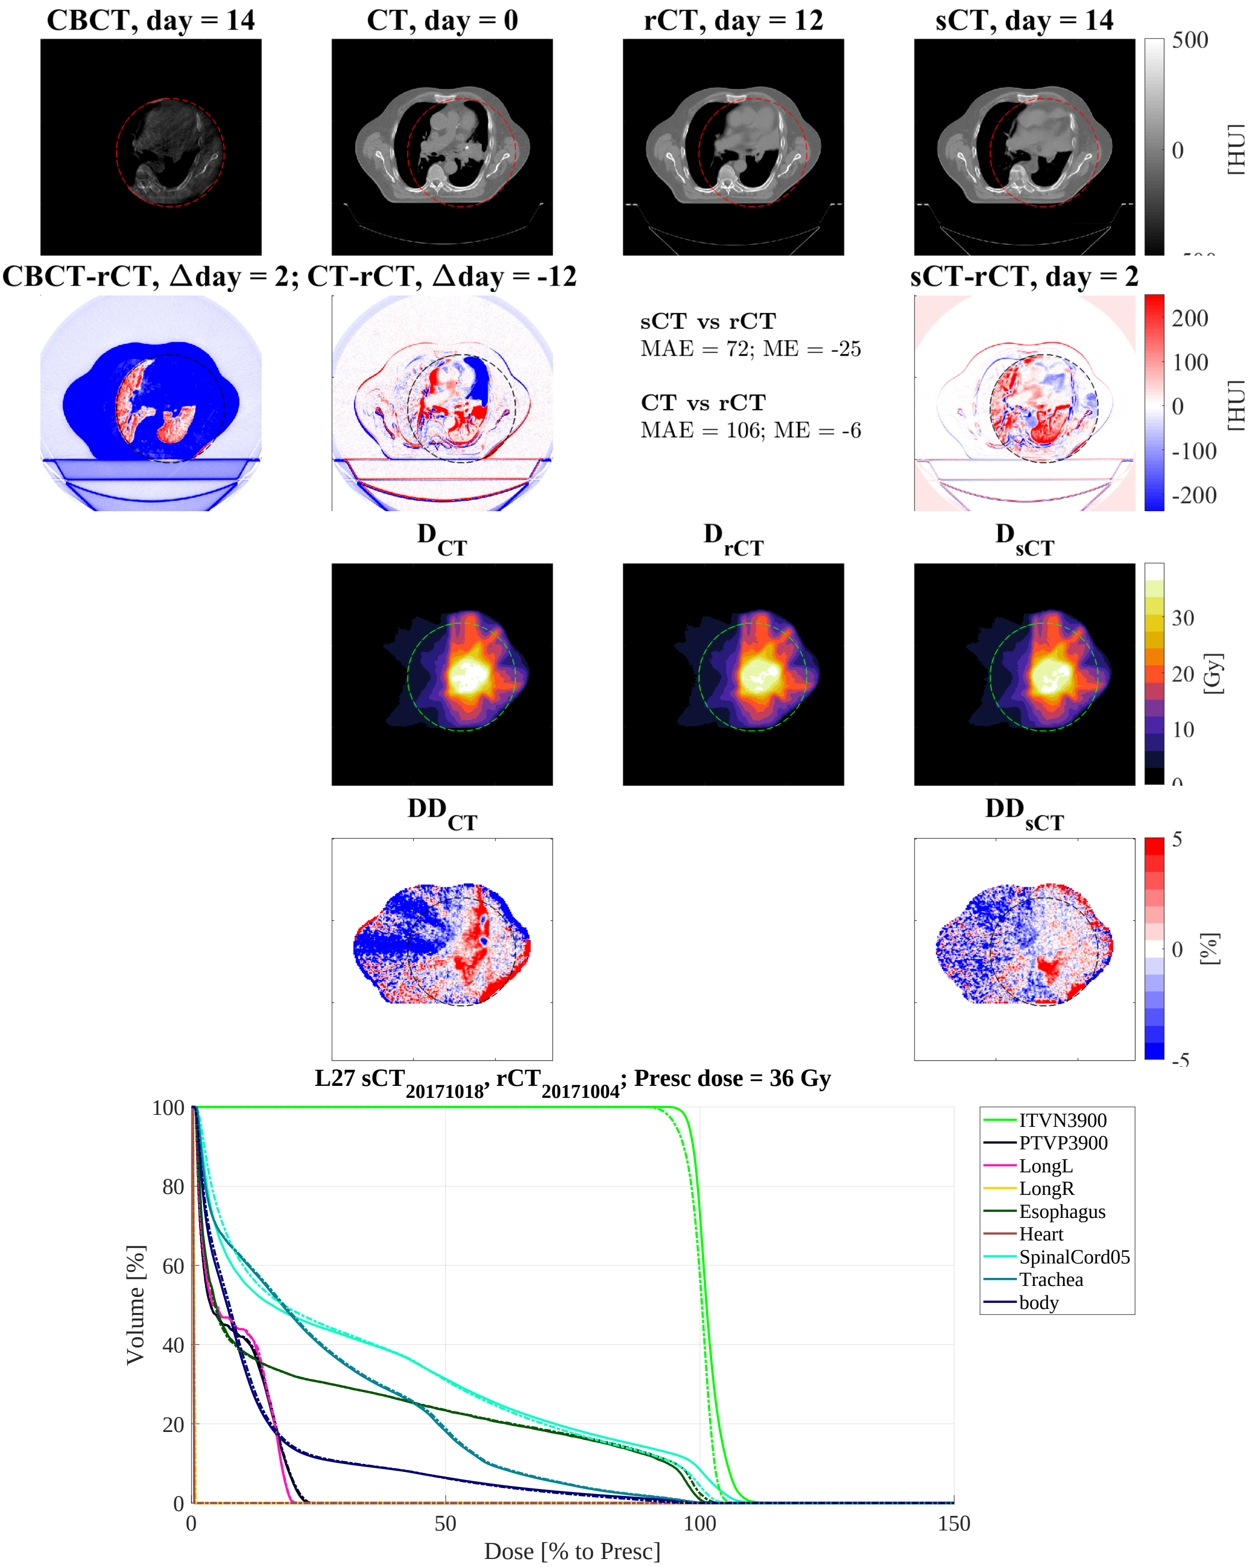


Figure 4: Axial views for the lung cancer patient L27 of: (1st row) CBCT (1st column), CT (2nd column), rescan CT (rCT, 3rd column) and synthetic CT (sCT, 4th column), along with (2nd row) the respective difference to rCT, the doses (3rd row) and the relative dose differences (4th). The red, black, or green dotted rectangles indicate the position of $\mathrm{Mask_{CBCT}}$. The days refer to the acquisition date of the rCT. In the 5th row, the DVH is shown for target and OARs of sCT (continuous lines) and rCT (dashed lines).
